# Supplementary material for: A Generalized Eulerian-Lagrangian Discontinuous Galerkin Method for Transport Problems
Source: arXiv:2102.11383 source file (2021-02-22)
Supplement: Supplementary file 1 [file appendix.tex]

%\begin{appendix}
\section{Search intersection points between quadratic-curved sides of an upstream cell and background grid lines}
\label{append:a}
The algorithm for searching intersection points between an upstream cell and the grid line $x= x_i$ is described in the following. The procedure for searching intersection points between the upstream cell and $v= v_j$ is pretty similar, thus omitted for brevity. 
%  \begin{description}
%    \item[Case 1.] 
    We can find intersection points of the quadratic curve determined by points $(x^\star_1,v^\star_1)$, $(x^\star_2,v^\star_2)$, $(x^\star_3,v^\star_3)$  and grid line $x=x_i$ by solving the following equation,
         \begin{equation}
     \begin{cases}
     x_i =   \frac{x^\star_3 -x^\star_1 }{2} \xi + \frac{v^\star_3 -v^\star_1 }{2} \eta
       + \frac{ x^\star_3 +x^\star_1 }{2}  , \\
      \eta = \frac{\eta_2}{ \xi_2^2-1 }(  \xi^2-1  ).
     \end{cases}
     \label{x_i}
     \end{equation}

     \begin{description}
       \item[Case 1]
       If $|x^\star_3- x^\star_1| \leq |v^\star_3 - v^\star_1| $, we have the following equation derived from \eqref{x_i},
       \begin{equation}
         A\xi^2 +  B\xi +C
       =0.
       \label{xi_quadratic}
       \end{equation}
    where
       \begin{align*}
       A&= \frac{\eta_2}{ \xi_2^2 - 1 }, \quad
       B= \frac{ x^\star_3 -x^\star_1 }{ v^\star_3 -v^\star_1 }, \quad
       C= - \frac{ \left(x_i -\frac{x^\star_1+x^\star_3}{2}\right) }{  \frac{v^\star_3-v^\star_1}{2} } -\frac{\eta_2 }{ \xi_2^2 -1 }.
       \end{align*}

       We can solve \eqref{xi_quadratic} as follows:
       %Define $ \max_{ABC} = \max ( |A| , |B|, |C| ) $.
       
  \bigskip     
\fbox{
\begin{minipage}[htb]{0.9\linewidth}
         \begin{algorithmic}
  \IF{ $A\ge \varepsilon$, where $\varepsilon=10^{-13}$ }
      \STATE
      Let
      $\Delta = B^2 -4AC$.

      If $\Delta<0$, there is no solution.

      If $\Delta=0$, there is only one solution,
%      \begin{equation}
      $\xi_1 = - \frac{B}{2A}.$
%      \end{equation}

      %%%%%%%%%%%%%%%%%%%%%%%%%%%%%%%%%%%%%%%%%%%%%%%%%%%%%%%%%%%%%%%%%%%%%%%%%%%%%%%%%%%%%%%%%%%%%%%%%
%      If $\Delta>0$ and $|-B - \gamma \sqrt{ B^2 - 4AC } | <2A$, where $\gamma=1$ if $B\geq 0$, and $\gamma=-1$ otherwise, there are two solutions,
%      \begin{equation}
%      \xi_{1,2} = \frac{ -B \pm \sqrt{ B^2 - 4AC } }{2A}.
%      %\xi_2 = \frac{ 2C }{ -B - \gamma \sqrt{ B^2 -4AC } },
%      \end{equation}
%
%      If $\Delta>0$ and $|-B - \gamma \sqrt{ B^2 - 4AC } | \geq 2A$, there are two solutions,
%      \begin{equation}
%      \xi_{1,2} = \frac{ -B - \gamma \sqrt{ B^2 - 4AC } }{2A},
%      \xi_2 = \frac{ 2C }{ -B - \gamma \sqrt{ B^2 -4AC } }.
%      \end{equation}
      %%%%%%%%%%%%%%%%%%%%%%%%%%%%%%%%%%%%%%%%%%%%%%%%%%%%%%%%%%%%%%%%%%%%%%%%%%%%%%%%%%%%%%%%%%%%%%%%%

%       If $\Delta>0$ and $|-B \pm \sqrt{ B^2 - 4AC } | \geq 2|A|$, there are two solutions,
%      \begin{equation}
%      \xi_{1,2} = \frac{ 2C }{ -B \pm \sqrt{ B^2 -4AC } }.
%      \end{equation}
%
%      And otherwise,
%      \begin{equation}
%      \xi_{1,2} = \frac{ -B \pm \sqrt{ B^2 - 4AC } }{2A}.
%      \end{equation}

       If $\Delta>0$, there are two solutions,
$$
      \xi_{1} =\frac{ 2C }{ -B - \gamma \sqrt{ \Delta } }, \quad
      \xi_2 =\frac{ -B - \gamma \sqrt{ \Delta } }{2A},
$$
      where $\gamma=1$ if $B\geq 0$, and $\gamma=-1$ otherwise.
 \ELSIF{ $A<\varepsilon$ and $B \ge \varepsilon$ }
  \STATE there is only one solution, $\xi_1 = - \frac{C}{B}.$
  \ELSE
  \STATE We retreat this case as no intersection points.

%  \IF{ $A =0, B=0$ and $C=0$, }
%    \STATE there are infinitely many solutions.
%  \ELSIF{ $A =0, B=0$ and $C\neq0$, }
%    \STATE there is no solution.
%  \ELSIF{ $A=0$ and $B\neq 0$,}
%    \STATE there is only one solution,
%    \begin{equation}
%     \xi_1 = - \frac{C}{B}.
%    \end{equation}

  \ENDIF
  
       If $\xi\in[-1,1]$, the solution $(\xi,\eta)$ is identified as an intersection point.
\end{algorithmic}
\end{minipage}
}

       \item[Case 2]
 If $|x^\star_3- x^\star_1| > |v^\star_3 - v^\star_1| $, we have the following equation derived from \eqref{x_i},
       \begin{equation*}
       A\eta^2 +B\eta +C =0,
       \end{equation*}
       where
       \begin{align*}
       A&= \frac{\eta_2}{\xi_2^2 - 1} \left( \frac{v^\star_3-v^\star_1}{x^\star_3-x^\star_1} \right)^2,\\
       B&=   -1- \frac{ 4\left(x_i-\frac{x^\star_1+x^\star_3}{2} \right) }{ x^\star_2 -x^\star_1 } \frac{v^\star_3 -v^\star_1 }{x^\star_3 -x^\star_1} \frac{ \eta_2 }{\xi_2^2-1},\\
       C&= \frac{\eta_2}{\xi_2^2 - 1}
       \left(  \frac{ 4\left( x_i - \frac{x^\star_1+x^\star_3}{2} \right)^2 }{ (x^\star_3 -x^\star_1)^2 }  -1 \right).
       \end{align*}

       Similar to Case 1.1, the solution $\eta$ can be solved. And then,
       \begin{equation}
       \xi = \frac{ 2x_i - x^\star_3 - x^\star_1 }{ x^\star_3 - x^\star_1 } - \frac{ v^\star_3 -v^\star_1 }{x^\star_3 -x^\star_1}\eta.
       \end{equation}

       If $\xi\in[-1,1]$, the solution $(\xi,\eta)$ is identified as an intersection point.

     \end{description}
